# Supplementary material for: SIMS: Simulating Stylized Human-Scene Interactions with Retrieval-Augmented Script Generation
Source: arXiv:2411.19921 source file (2025-03-16)
Supplement: Supplementary file 1 [file supp_dataset_statistics.tex]

\begin{table}[]
    \centering
    \begin{tabular}{c|c}
         &  \\
         & 
    \end{tabular}
    \caption{Caption}
    \label{tab:dataset_statistics}
\end{table}
